# Supplementary material for: Optimal Reward Allocation via Proportional Splitting
Source: arXiv:2503.10185 source file (2026-08-10)
Supplement: Supplementary file 1 [file appendix.tex]

\section{Relevant Literature Protocols}\label{app:literature-protocols}

\subsection{PoEM}

PoEM~\cite{poem} is a variant of Bitcoin, which modifies the fork choice rule.
Apart from this change, the main protocol's routine (Algorithm~\ref{alg.poem}) and
the PoW mechanism (Algorithm~\ref{alg.poem-pow}) are the same as Bitcoin.

In Bitcoin, the fork choice rule states that honest parties adopt the longest chain.
Specifically, when validating a chain, a party checks whether each block in the chain
satisfies the PoW inequality (for the given threshold). Following, among all valid
chains, the party picks the one with the most blocks, \ie the longest.

In PoEM, parties adopt the chain with the most amount of ``intrinsic work''
(Algorithm~\ref{alg.poem-maxvalid}).
Here, a block $\block$'s intrinsic work is defined as $-\log \frac{\hash(\block)}{T}$, 
where $\hash(\block)$ is $\block$'s hash and $T$ is the PoW threshold. Intuitively,
the intrinsic work counts the number of zeroes at the beginning of a block's hash.
As opposed to Bitcoin, where a block's work is computed as $-\log T$, in PoEM a block
with more zeroes at the beginning of its hash is prioritized. Equivalently,
a chain's (approximate) intrinsic work (denoted by $\awork(\chain)$)
is computed as the sum of the intrinsic work of all its blocks.

\begin{algorithm}
    \caption{\label{alg.poem} The PoEM protocol}
    \begin{algorithmic}[1]
        \Statex
        \State{$\genesis$}
        \Let{\chain}{[\,]}
        \Function{$\constructor$}{$\genesis'$}\label{alg-backbone.constructor}
            \State $\genesis \leftarrow \genesis'$ \Comment{Select Genesis Block}
            \State $ \chain \leftarrow [\genesis]$ \Comment{Add Genesis Block to start of chain}
            \State \textsf{round} $\leftarrow 1$
        \EndFunction
        \Function{$\execute_{\net}$}{$1^\secparam$}
            \CommentLine{Receive chains from the network}
            \State $\bar M \leftarrow \net.\receive()$
            \State $\chain \leftarrow \maxvalid(\{ \chain \} \cup \bar M)$ \Comment{Adopt heaviest chain}
            \Let{x}{\textsc{input}()} \Comment{Take all transactions in mempool}
            \Let{\block}{\pow(x, \aH(\chain[-1]))} \Comment{Mine a new block}
            \If{$\block \neq \bot$} \Comment{Successful mining}
                \State $\net.\broadcast(\chain \concat \block)$ \Comment{Broadcast mined chain}
            \Else
                \State $\net.\broadcast(\chain)$ \Comment{Broadcast adopted chain}
            \EndIf
            \State {\textsf{round}} $\leftarrow$ {\textsf{round}+1}
        \EndFunction
    \end{algorithmic}
\end{algorithm}

\begin{algorithm}[h]
    \caption{\label{alg.poem-pow} The PoEM Proof-of-Work mechanism}
    \begin{algorithmic}[1]
        \Function{$\pow_{H,T,q}$}{$x, h$}
            \State{$\nonce \getsrandomly \{0,1\}^\secparam$}
            \For{$i \gets 1 \text{ to } q$}
                \Let{\chain}{h \concat x \concat \nonce}
                \If{$\aH(\chain) < T$}
                    \State\Return{$\chain$}
                \EndIf
                \Let{\nonce}{\nonce + 1}
            \EndFor
            \State \Return{$\bot$}
        \EndFunction
    \end{algorithmic}
\end{algorithm}

\begin{algorithm}[h]
    \caption{\label{alg.poem-maxvalid} The PoEM maxvalid algorithm}
    \begin{algorithmic}[1]
        \Function{$\maxvalid_{\genesis,T}$}{$\overline{\chain}$}
            \Let{\chain_\mmax}{[\,]}
            \Let{\maxwork}{0}
            \For{$\chain \in \overline{\chain}$}
                \If{$\lnot\validate_{\genesis}(\chain)$}
                    \Continue
                \EndIf
                \Let{\thiswork}{\awork(\chain)} \Comment{Computed as $\sum_{\block \in \chain} \hash(\block)_{:\secparam}$}
                \If{$\thiswork > \maxwork$}
                    \Let{\chain_\mmax}{\chain}
                    \Let{\maxwork}{\thiswork}
                \EndIf
            \EndFor
            \State \Return{$\chain_\mmax$}
        \EndFunction
    \end{algorithmic}
\end{algorithm}
